# Supplementary material for: A comprehensive analysis of differential cross sections and analyzing powers in the proton-deuteron break-up channel at 135 MeV
Source: arXiv:2008.12177 ancillary file (2020-08-27)
Supplement: Supplementary file 1 [file Supplementary_Material.pdf]

# Supplemental material

belonging to the paper

# A comprehensive analysis of differential cross sections and analyzing powers in the proton-deuteron break-up channel at 135 MeV

H. Tavakoli-Zaniani[1,2a], M. Eslami-Kalantari[2b], H. R. Amir-Ahmadi[1], M. T. Bayat[1], A. Deltuva[3], J. Golak[4], N. Kalantar-Nayestanaki[1], St. Kistryn[5], A. Kozela[6], H. Mardanpour[1], J. G. Messchendorp[1c], M. Mohammadi-Dadkan[1,7], A. Ramazani-Moghaddam-Arani[8], R. Ramazani-Sharifabadi[1,9], R. Skibiński[4], E. Stephan[10], and H. Witała[4]

[1] KVI-CART, University of Groningen, Groningen, the Netherlands
[2] Department of Physics, School of Science, Yazd University, Yazd, Iran
[3] Institute of Theoretical Physics and Astronomy, Vilnius University, Lithuania
[4] M.Smoluchowski Institute of Physics, Jagiellonian University, Kraków, Poland
[5] Institute of Physics, Jagiellonian University, Kraków, Poland
[6] Institute of Nuclear Physics, PAS, Kraków, Poland
[7] Department of Physics, University of Sistan and Baluchestan, Zahedan, Iran
[8] Department of Physics, Faculty of Science, University of Kashan, Kashan, Iran
[9] Department of Physics, University of Tehran, Tehran, Iran
[10] Institute of Physics, University of Silesia, Chorzów, Poland

**Experimental results:** Figures 1– 20 show the results of the cross sections and analyzing powers ($A_x$ and $A_y$) as a function of $S$ for about hundred configurations. The results of our analysis are indicated as black dots. The error bars indicate statistical uncertainties. In many cases, the cross-section statistical uncertainties are smaller than the symbol sizes. The cyan bands depict the systematical uncertainty whereby the width corresponds to $2\sigma$. The various lines present the results of Faddeev calculations using 2NF and 2N+3NF models such as CD-Bonn, red (dotted-dashed) line, CDB+$\Delta$, blue (dotted) line, and CDB+$\Delta$ including Coulomb effect (CDB+$\Delta$+Coulomb), black (solid) line from the Hannover-Lisbon group [1-3] and CDB+TM', green (double dotted-dashed) line, from the Bochum-Kraków group [4,5].

[a] h.tavakoli.zaniani@rug.nl
[b] meslami@yazd.ac.ir
[c] j.g.messchendorp@rug.nl

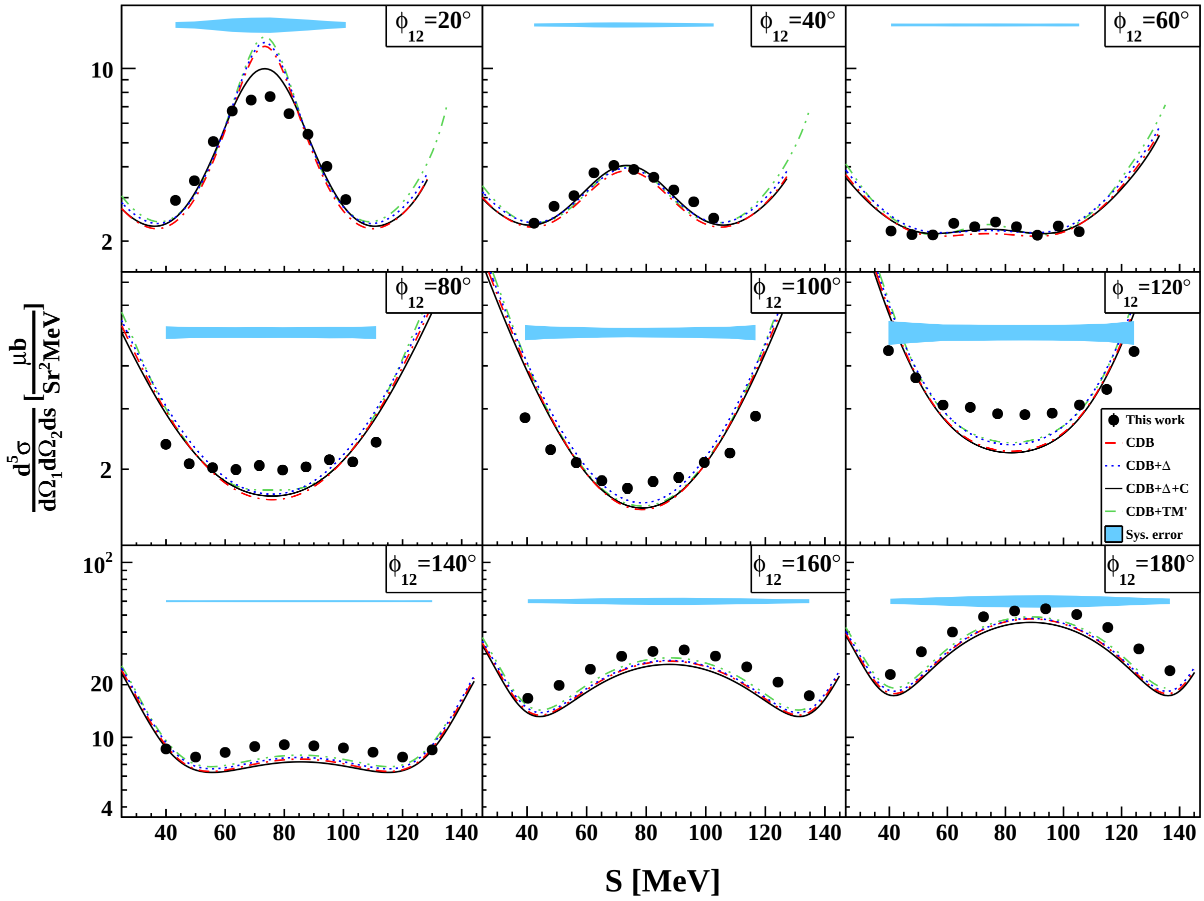


Fig. 1: The cross sections at (28°, 28°) as a function of $S$ at different azimuthal angles. Error bars show the statistical uncertainties for the data points. The red (dotted-dashed), blue (dotted), black (solid) and green (double dotted-dashed) lines show the predictions of Faddeev calculations using CD-Bonn, CDB+$\Delta$, and CDB+$\Delta$ including Coulomb and CDB+TM′ calculations [1-5], respectively. The cyan bands depict the systematic uncertainties ($2\sigma$).

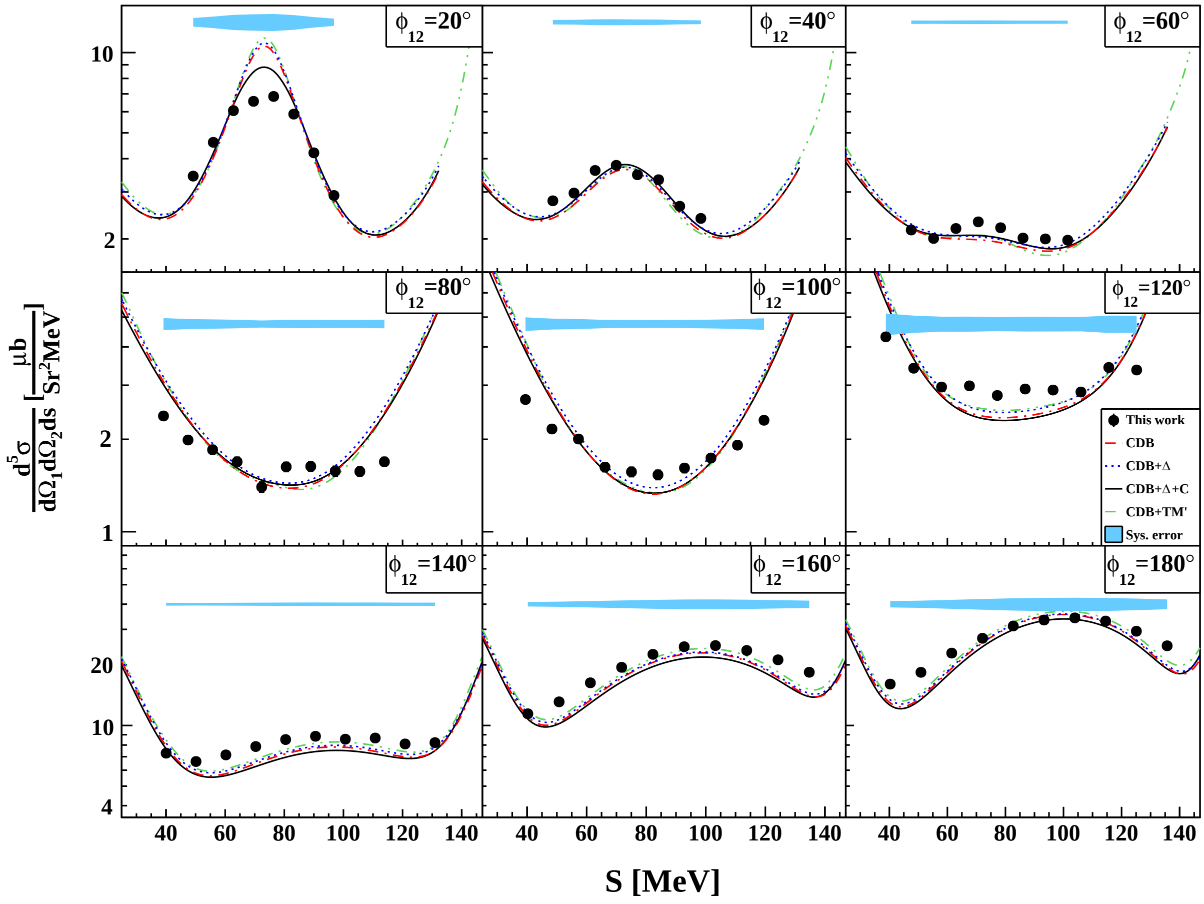


Fig. 2: Same as Fig. 1 except for $(\theta_1, \theta_2) = (28°, 24°)$.

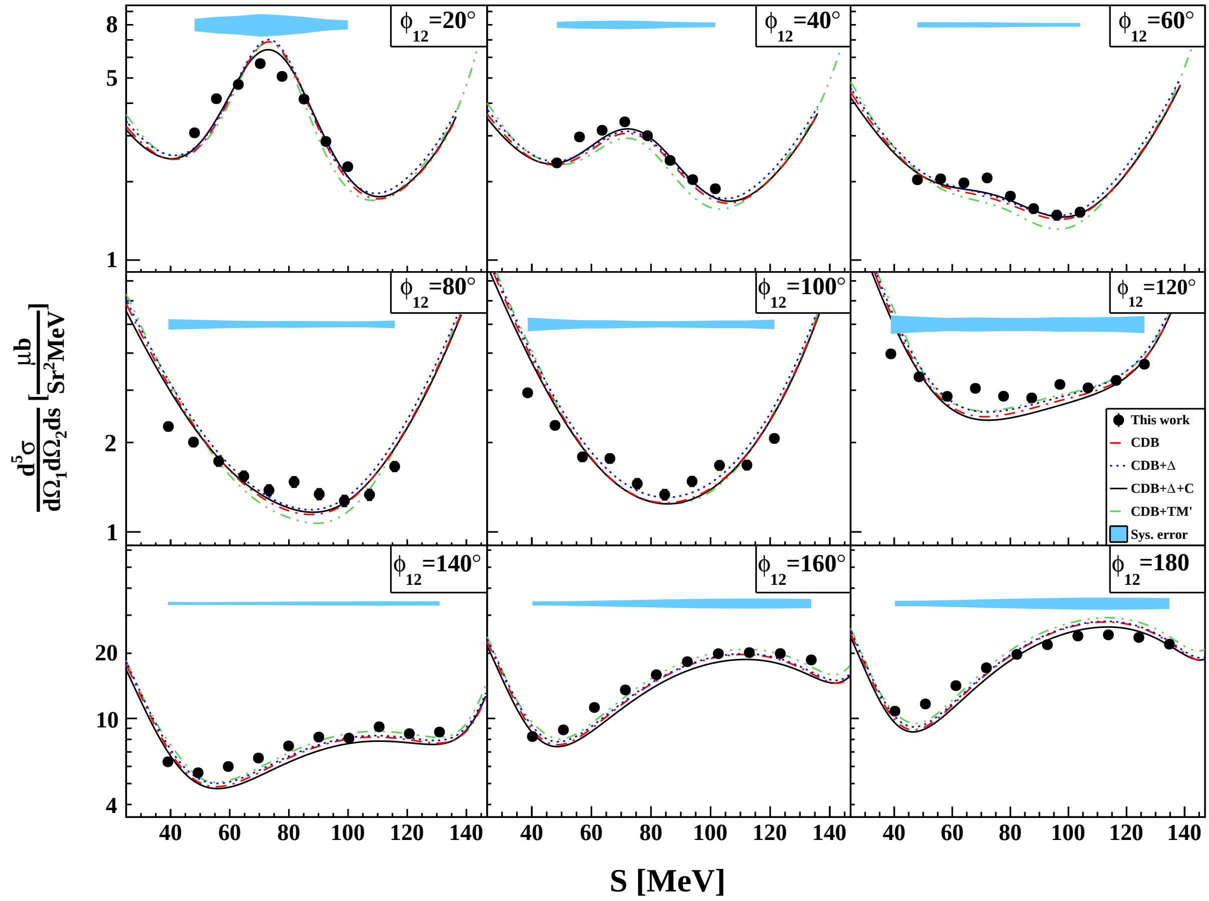


Fig. 3: Same as Fig. 1 except for $(\theta_1, \theta_2) = (28°, 20°)$.

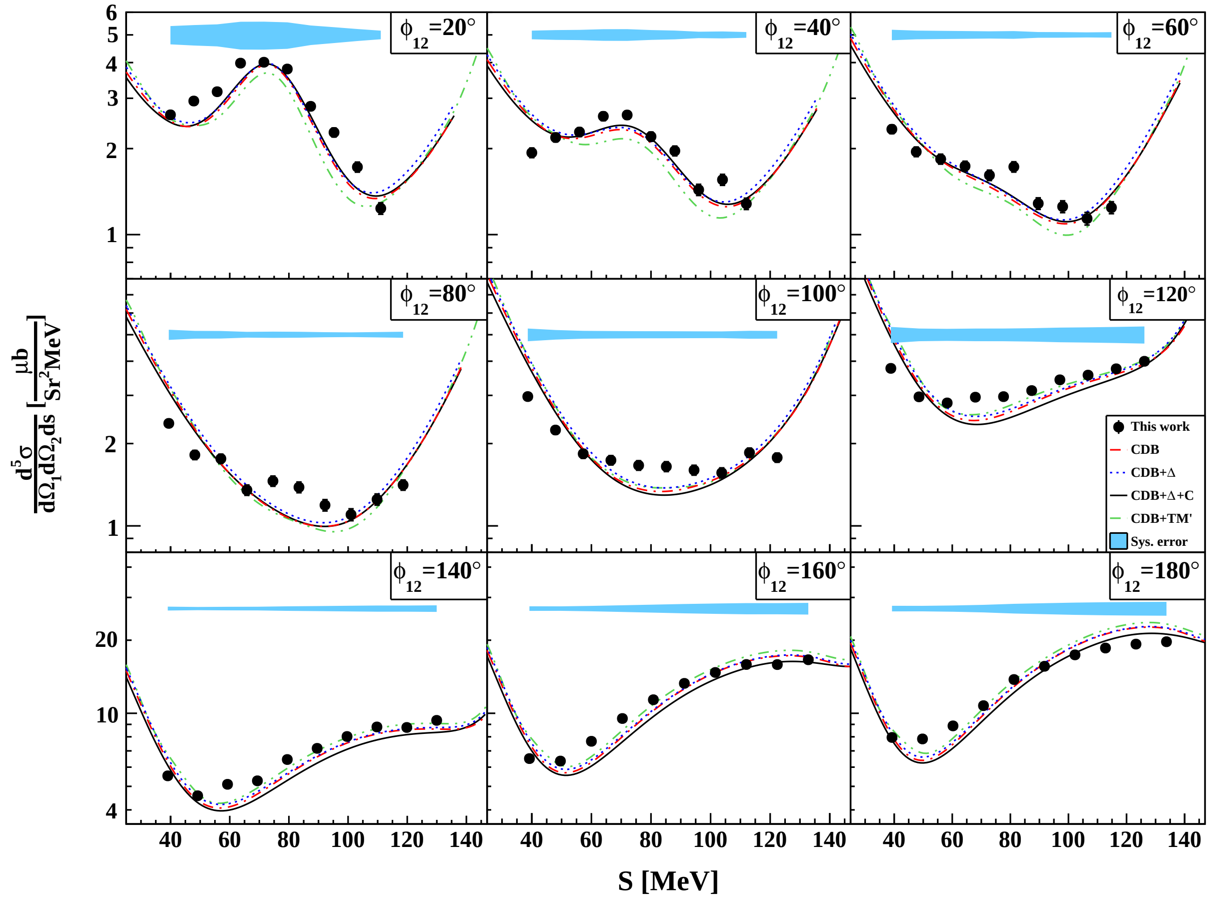


Fig. 4: Same as Fig. 1 except for $(\theta_1, \theta_2) = (28°, 16°)$.

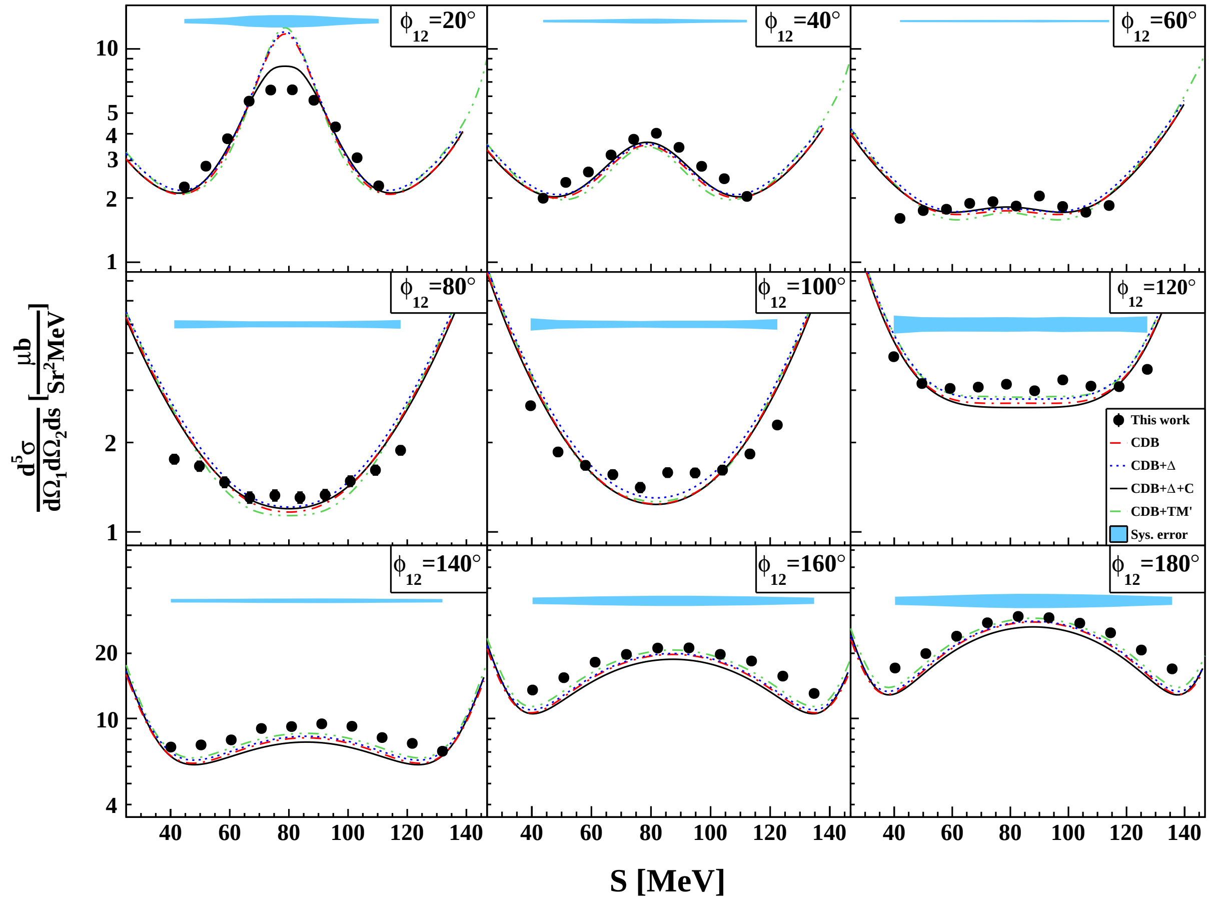


Fig. 5: Same as Fig. 1 except for $(\theta_1, \theta_2) = (24°, 24°)$.

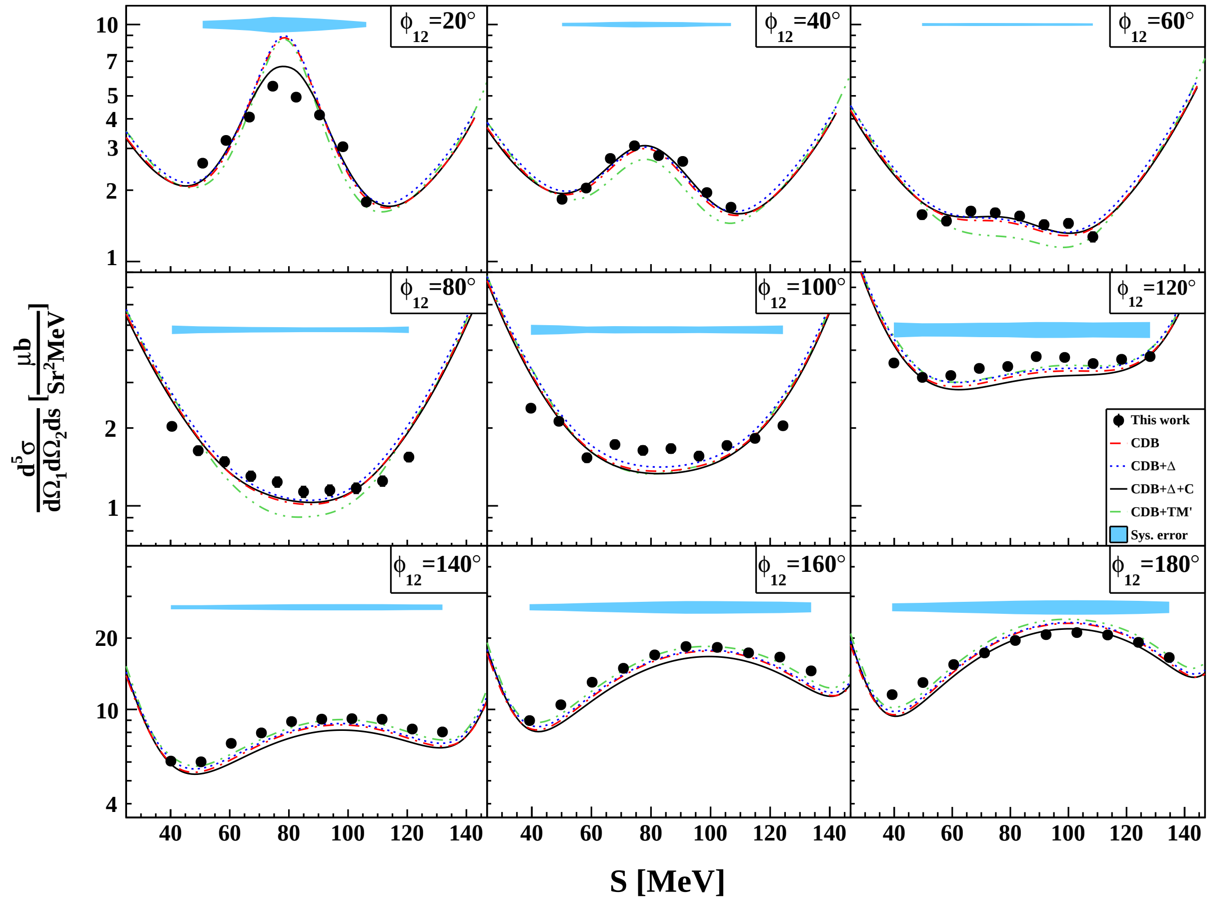


Fig. 6: Same as Fig. 1 except for $(\theta_1, \theta_2) = (24°, 20°)$.

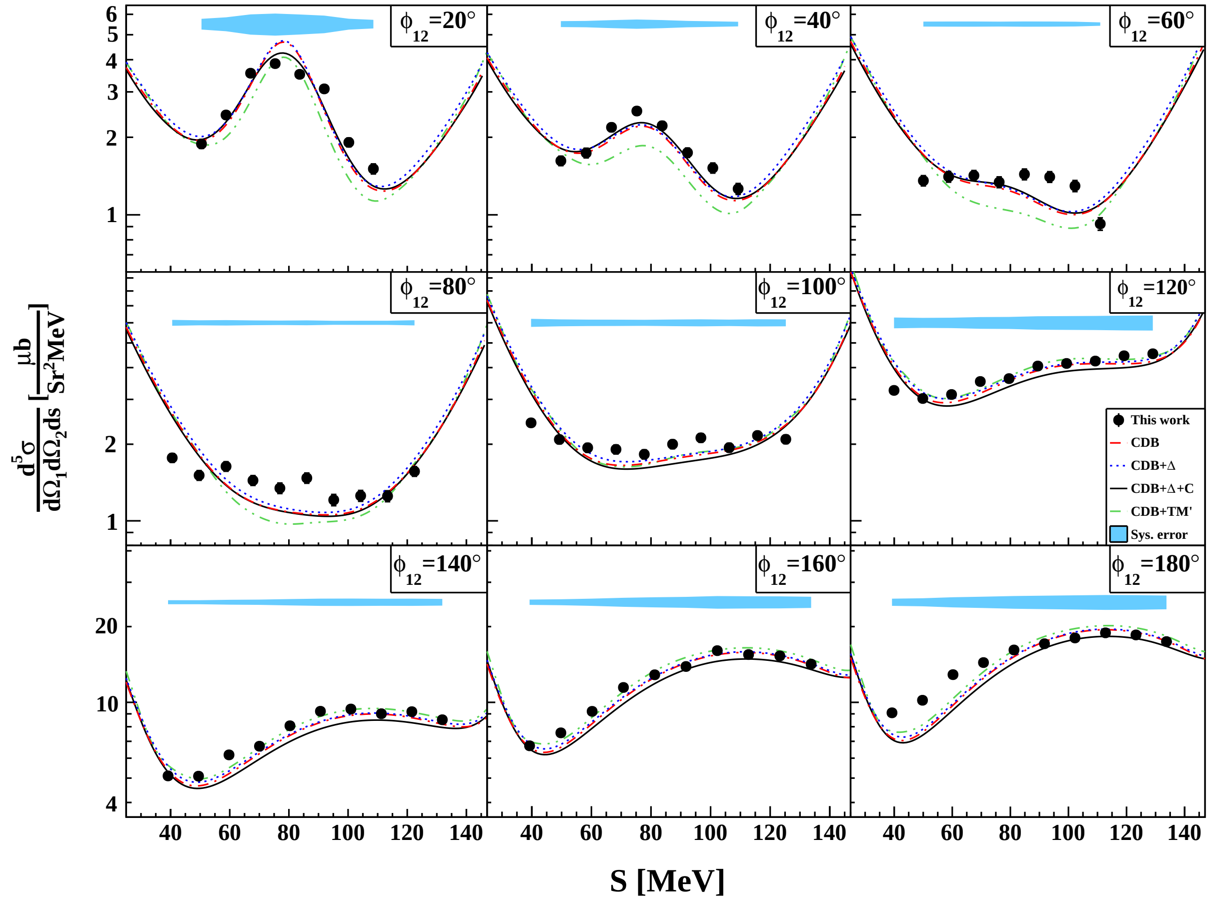


Fig. 7: Same as Fig. 1 except for $(\theta_1, \theta_2) = (24^\circ, 16^\circ)$.

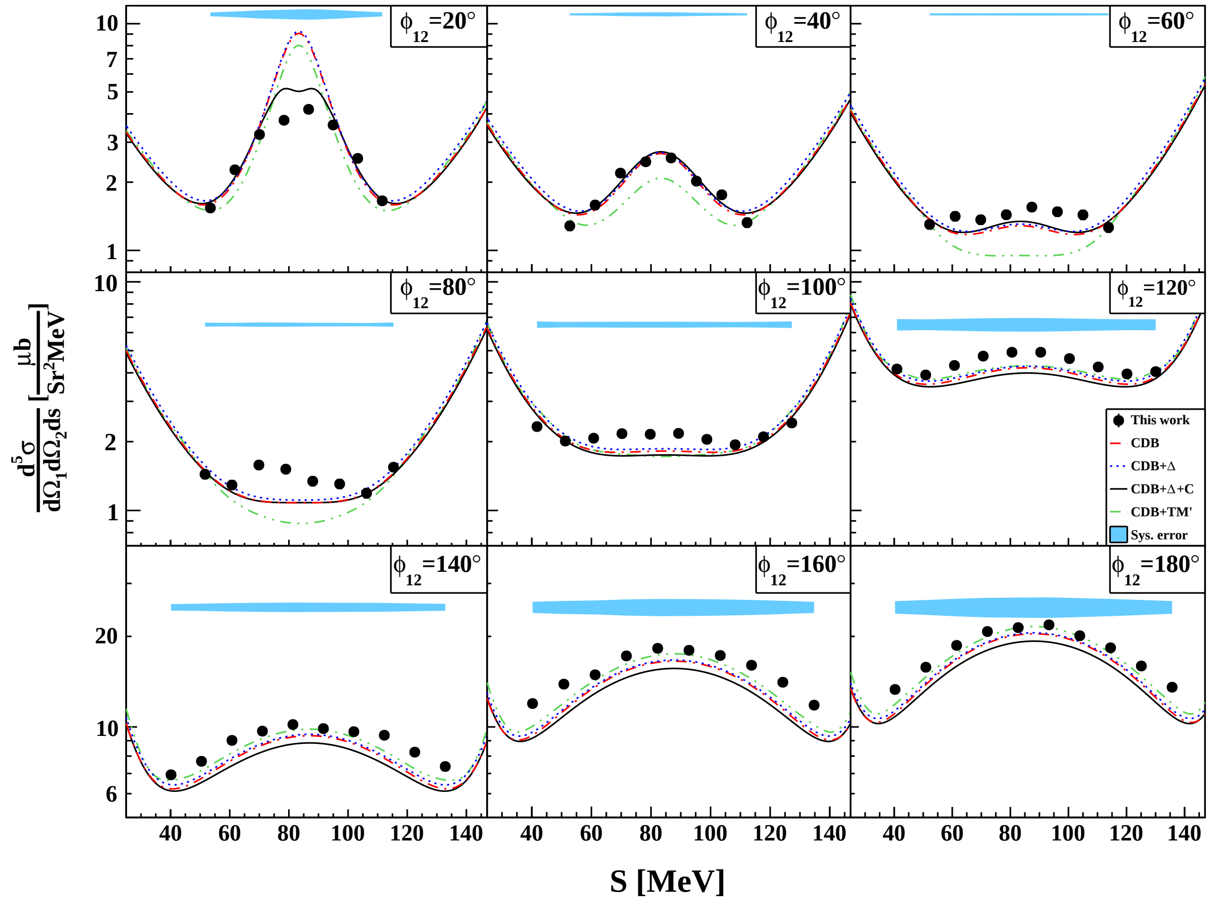


Fig. 8: Same as Fig. 1 except for $(\theta_1, \theta_2) = (20^\circ, 20^\circ)$.

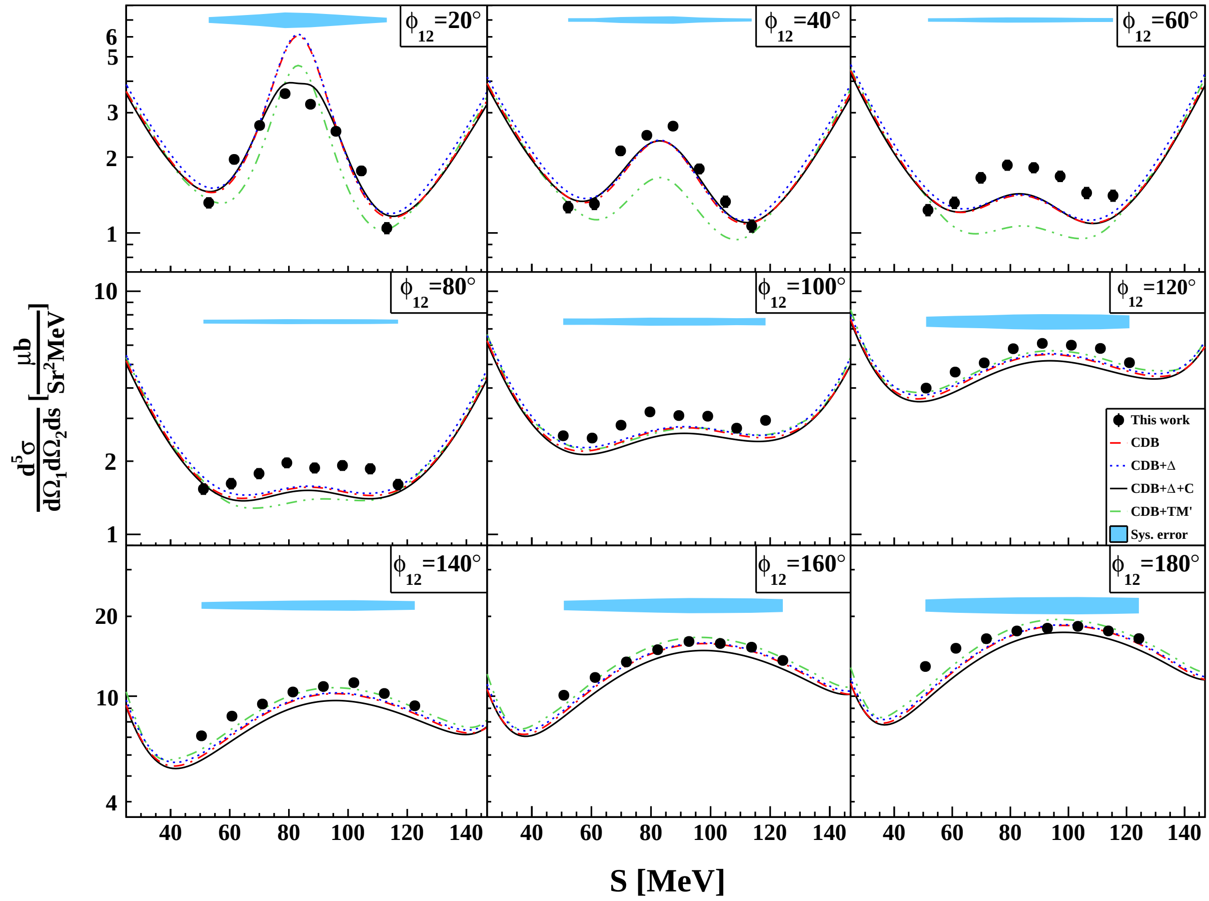


Fig. 9: Same as Fig. 1 except for $(\theta_1, \theta_2) = (20^\circ, 16^\circ)$.

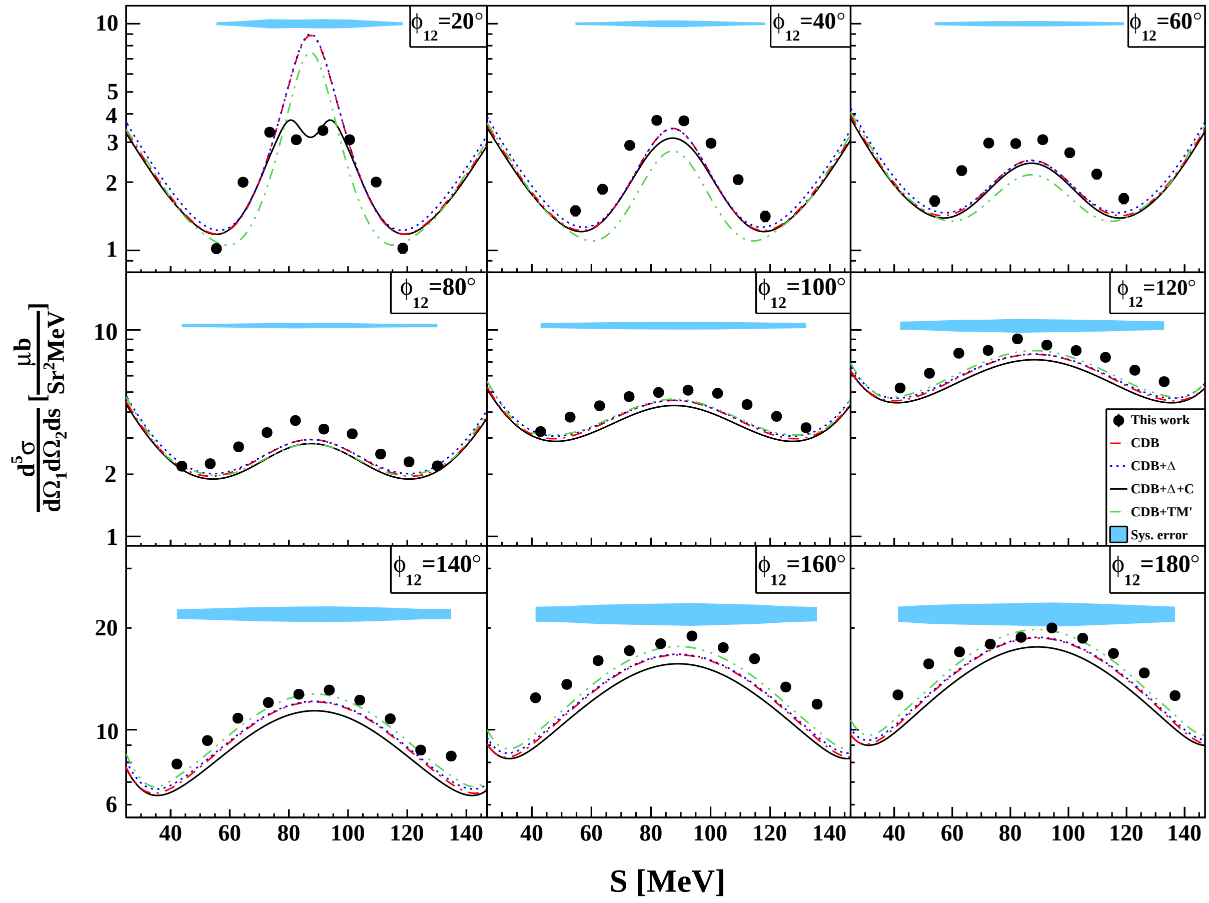


Fig. 10: Same as Fig. 1 except for $(\theta_1, \theta_2) = (16^\circ, 16^\circ)$.

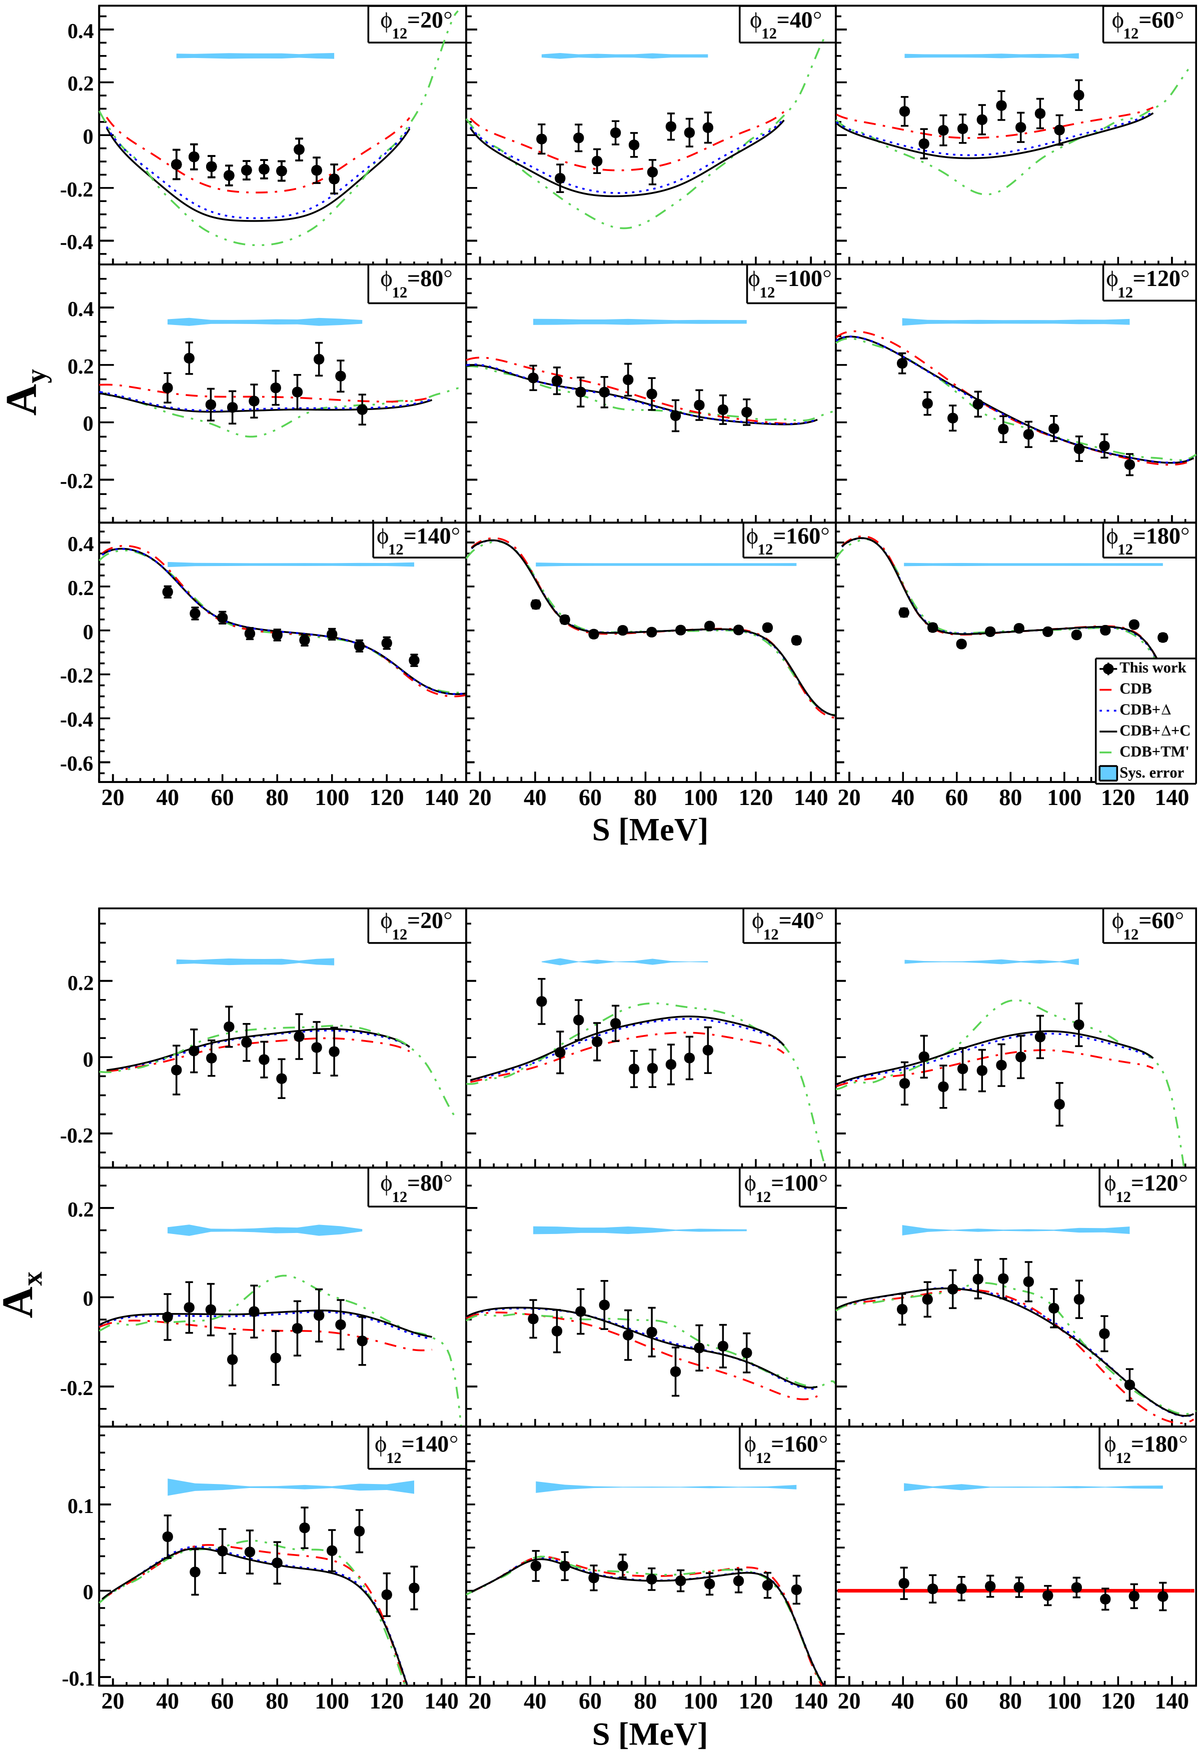


Fig. 11: Same as Fig. 1 for $(\theta_1, \theta_2) = (28^\circ, 28^\circ)$ except for $A_x$ and $A_y$. The red lines in the bottom panels correspond to a zero line.

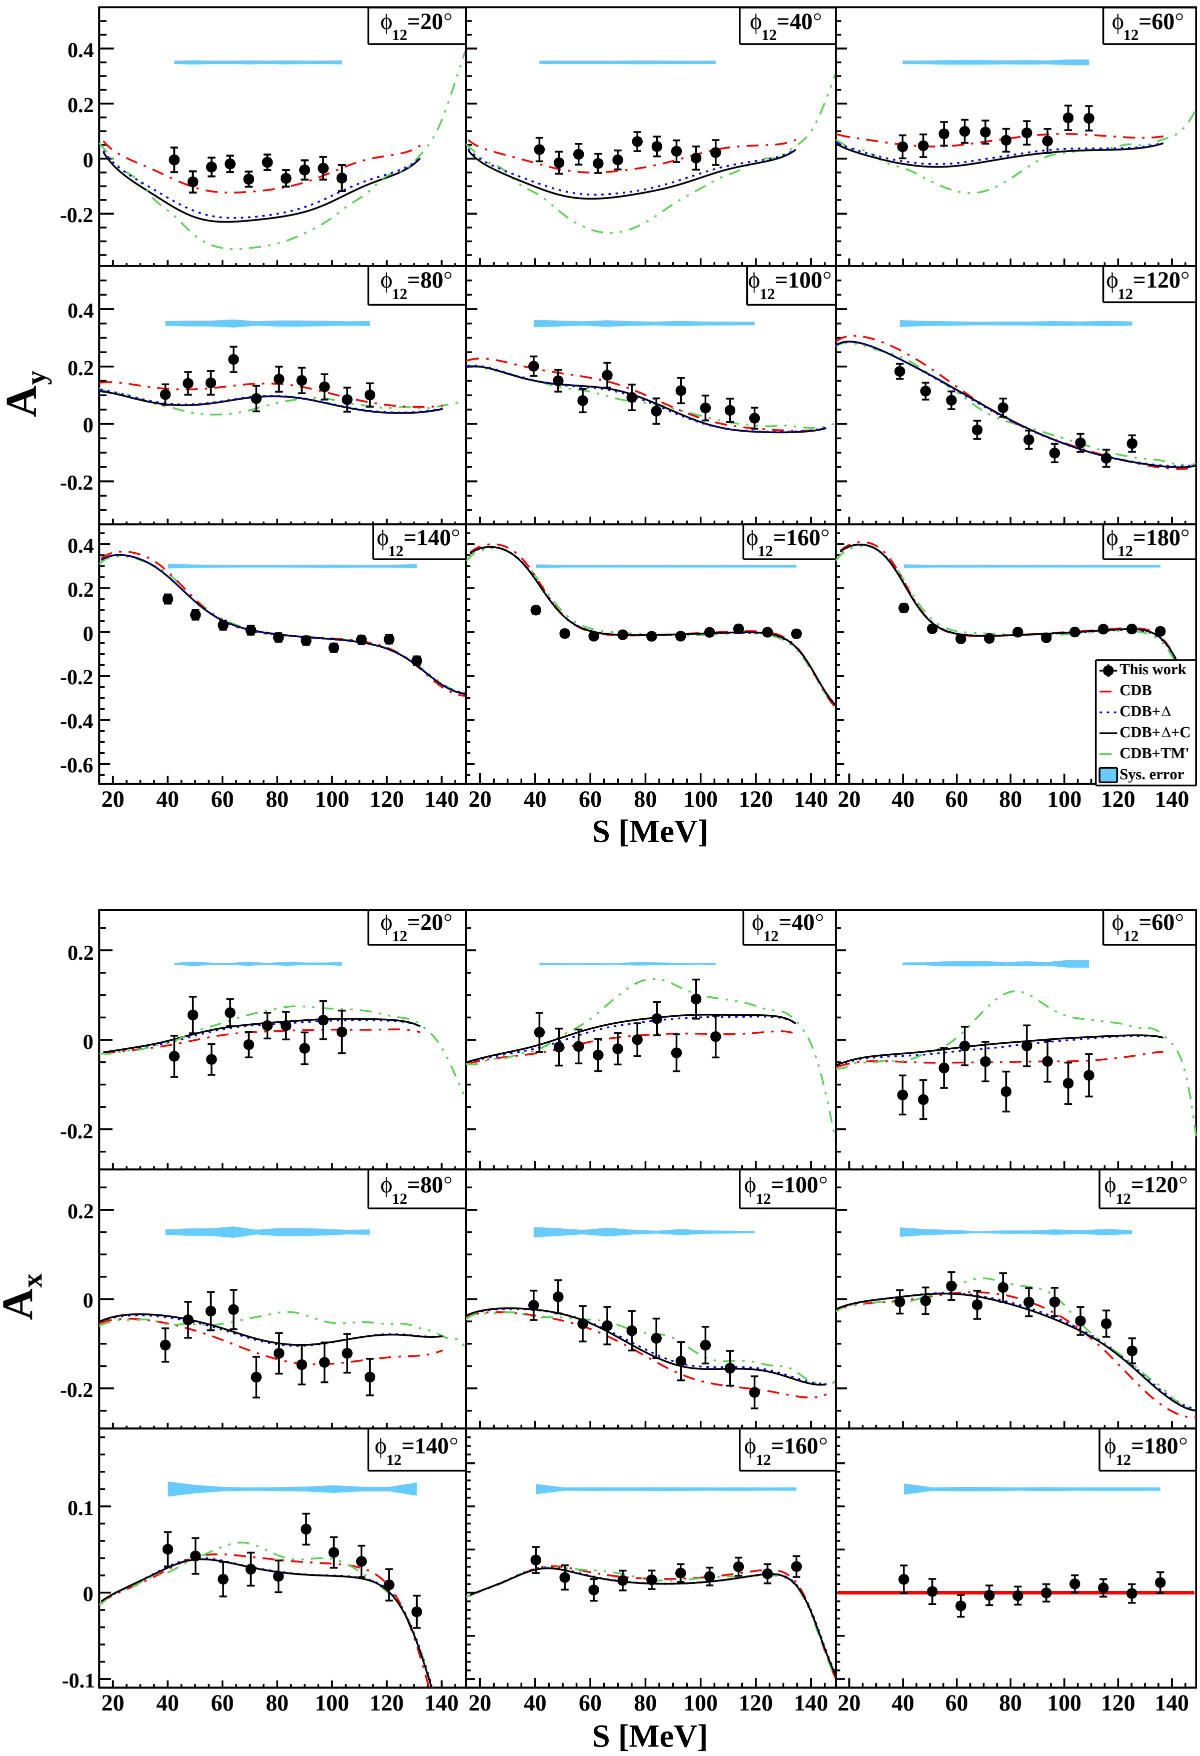


Fig. 12: Same as Fig. 11 except for $(\theta_1, \theta_2) = (28^{\circ}, 24^{\circ})$.

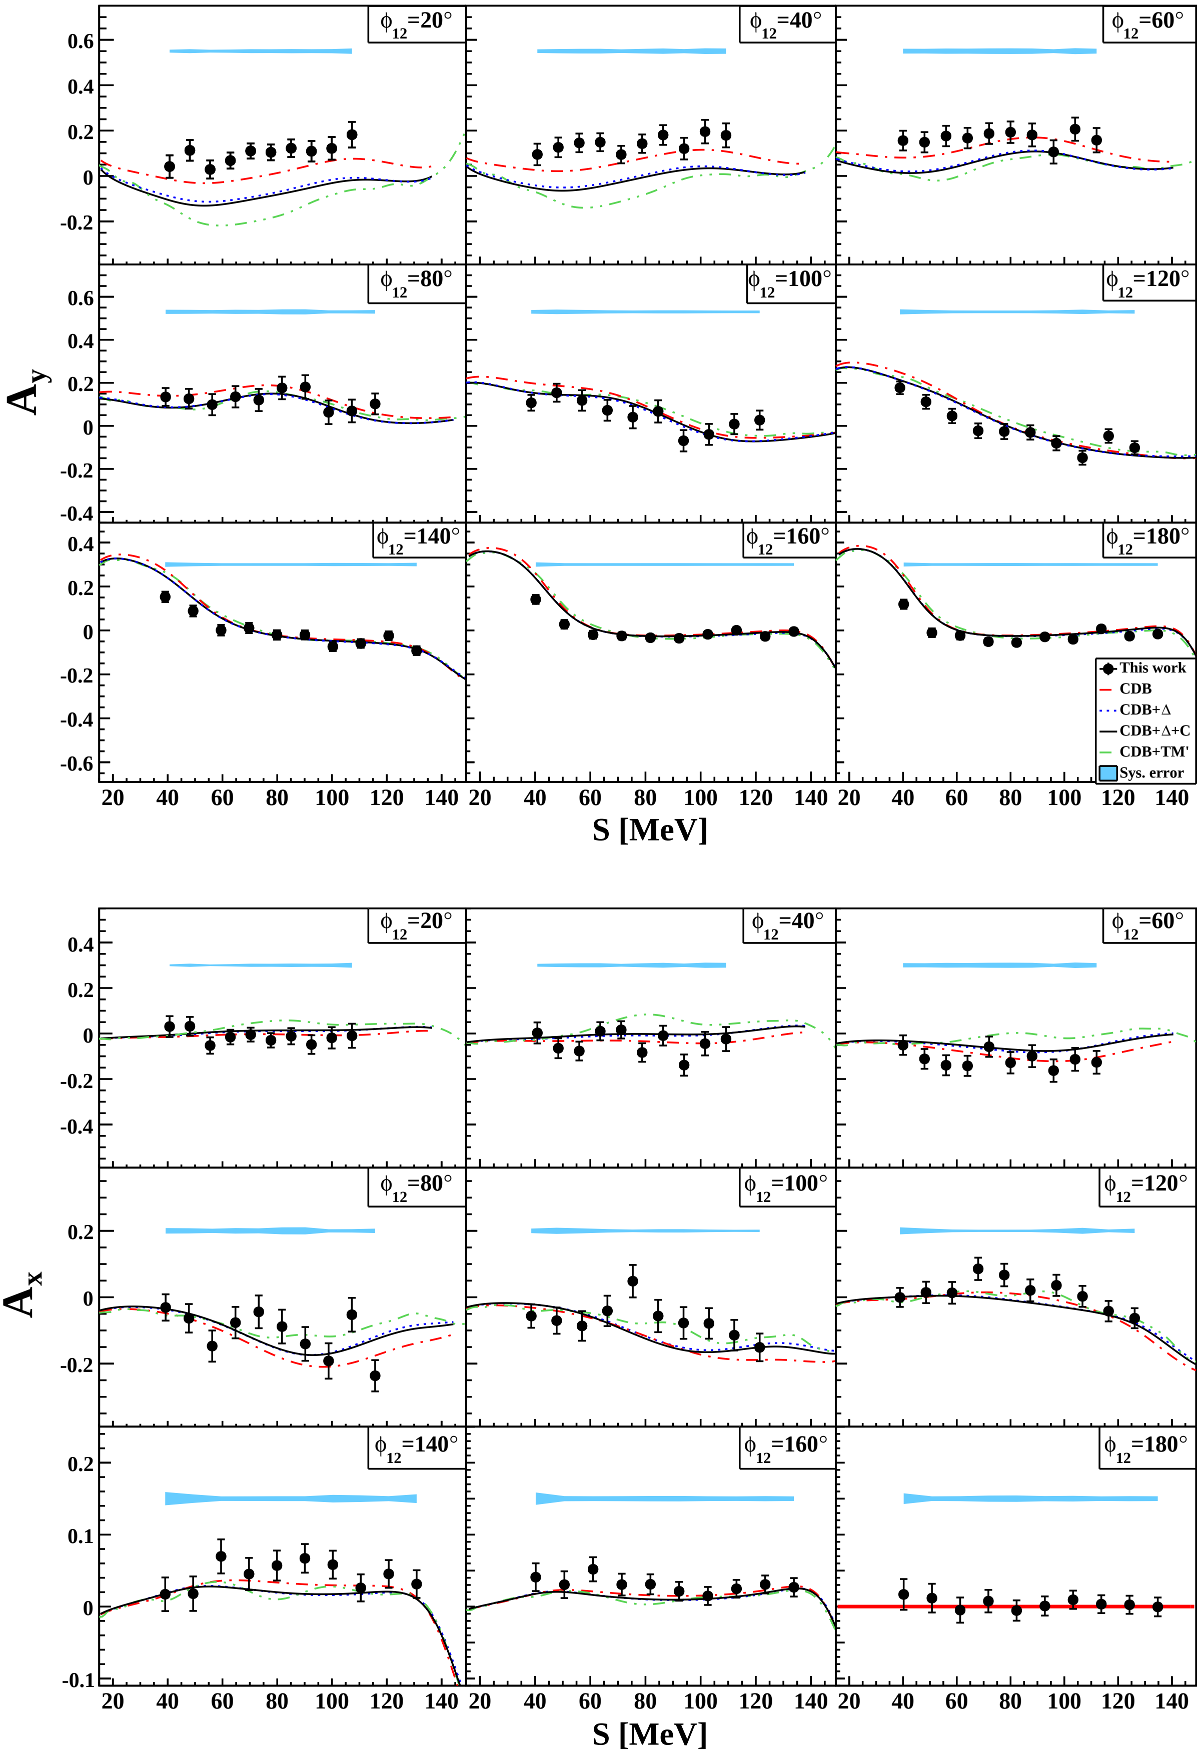


Fig. 13: Same as Fig. 11 except for $(\theta_1, \theta_2) = (28°, 20°)$.

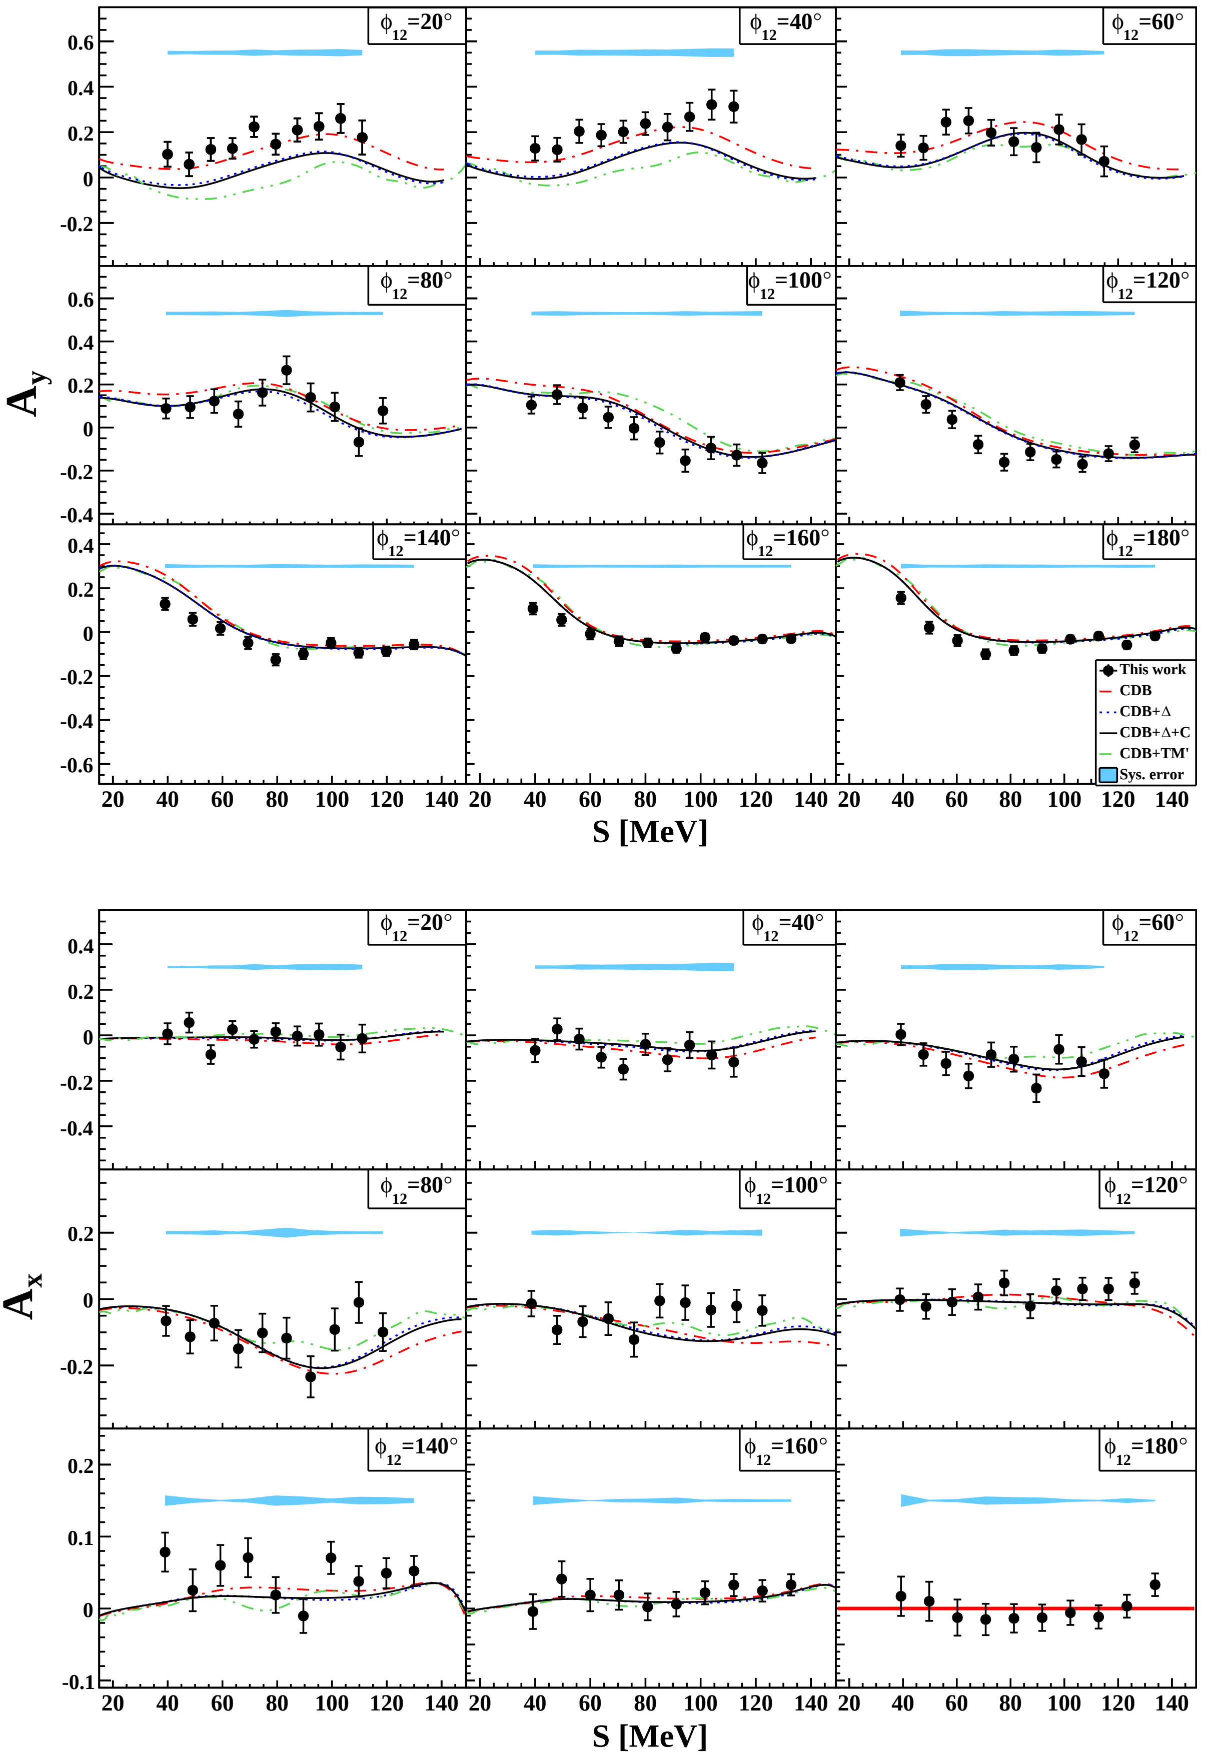


Fig. 14: Same as Fig. 11 except for $(\theta_1, \theta_2) = (28^\circ, 16^\circ)$.

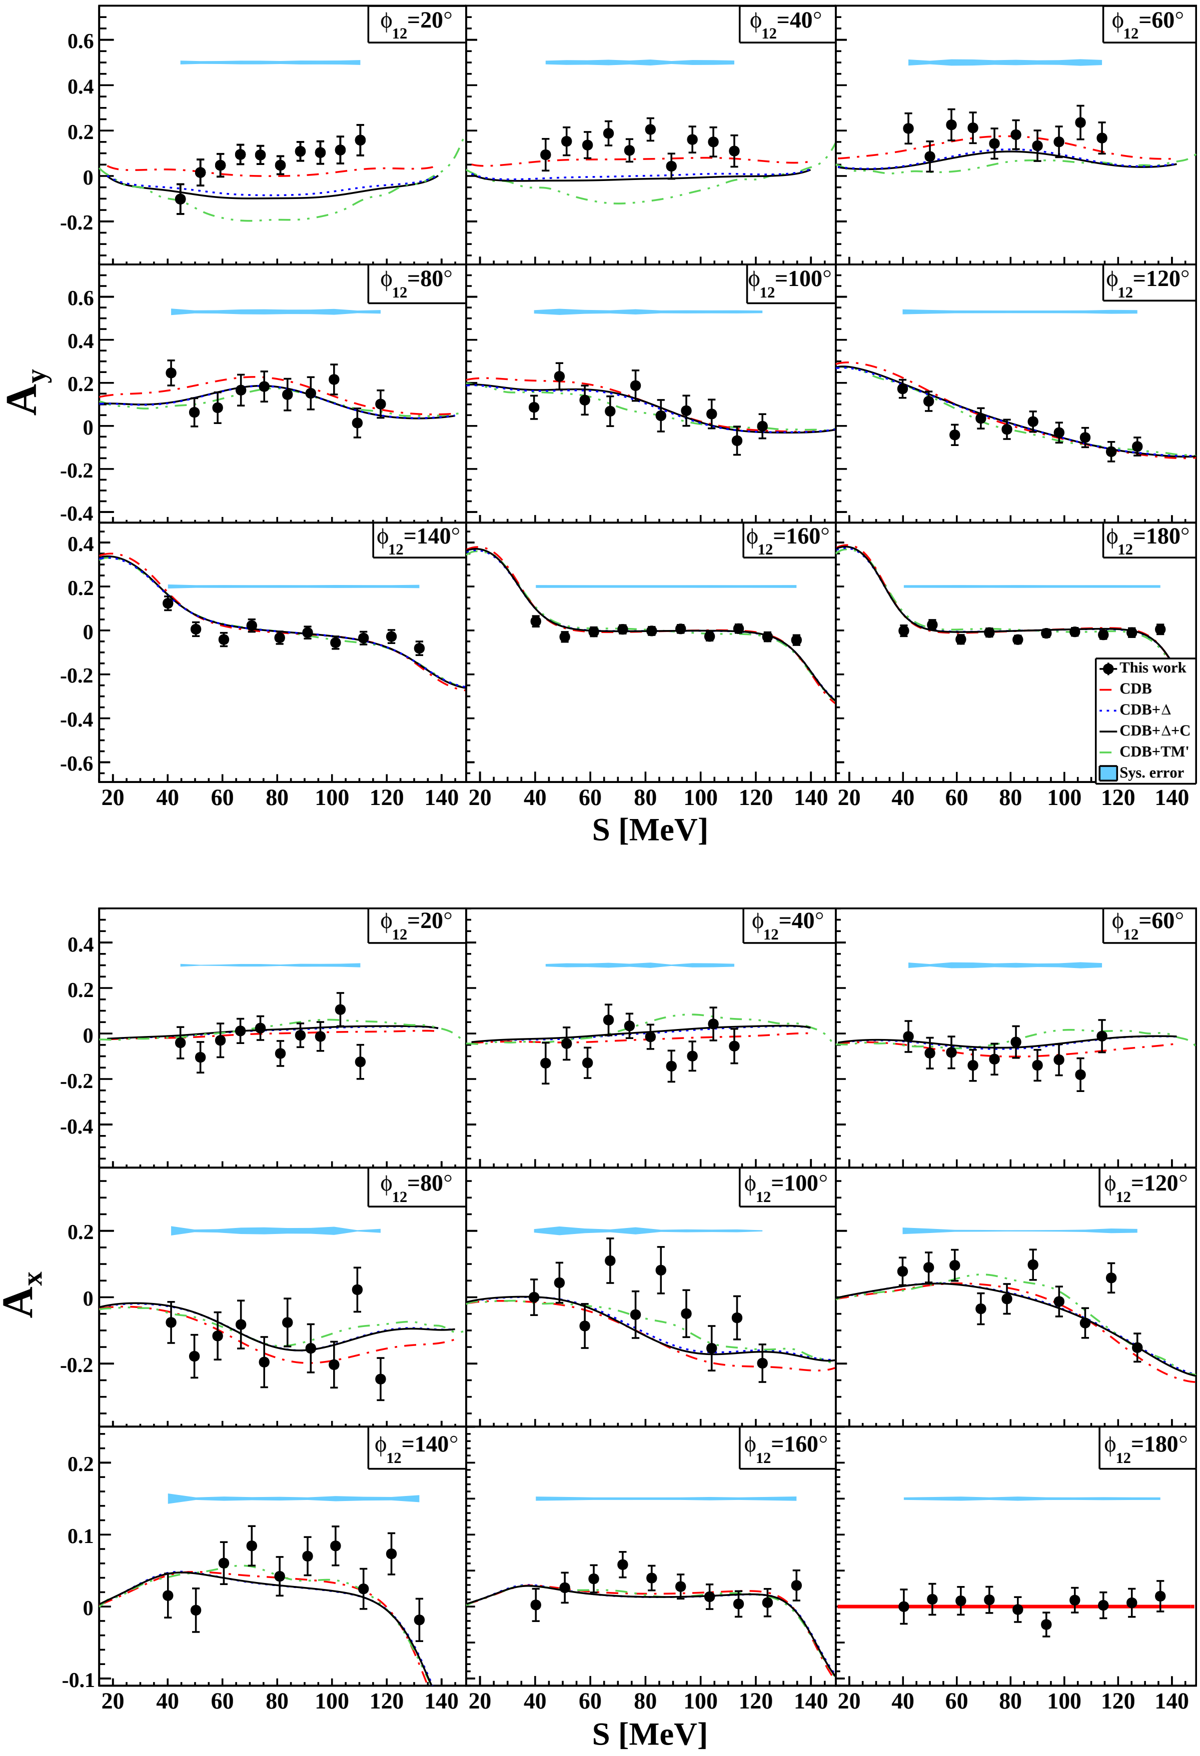


Fig. 15: Same as Fig. 11 except for $(\theta_1, \theta_2) = (24^\circ, 24^\circ)$.

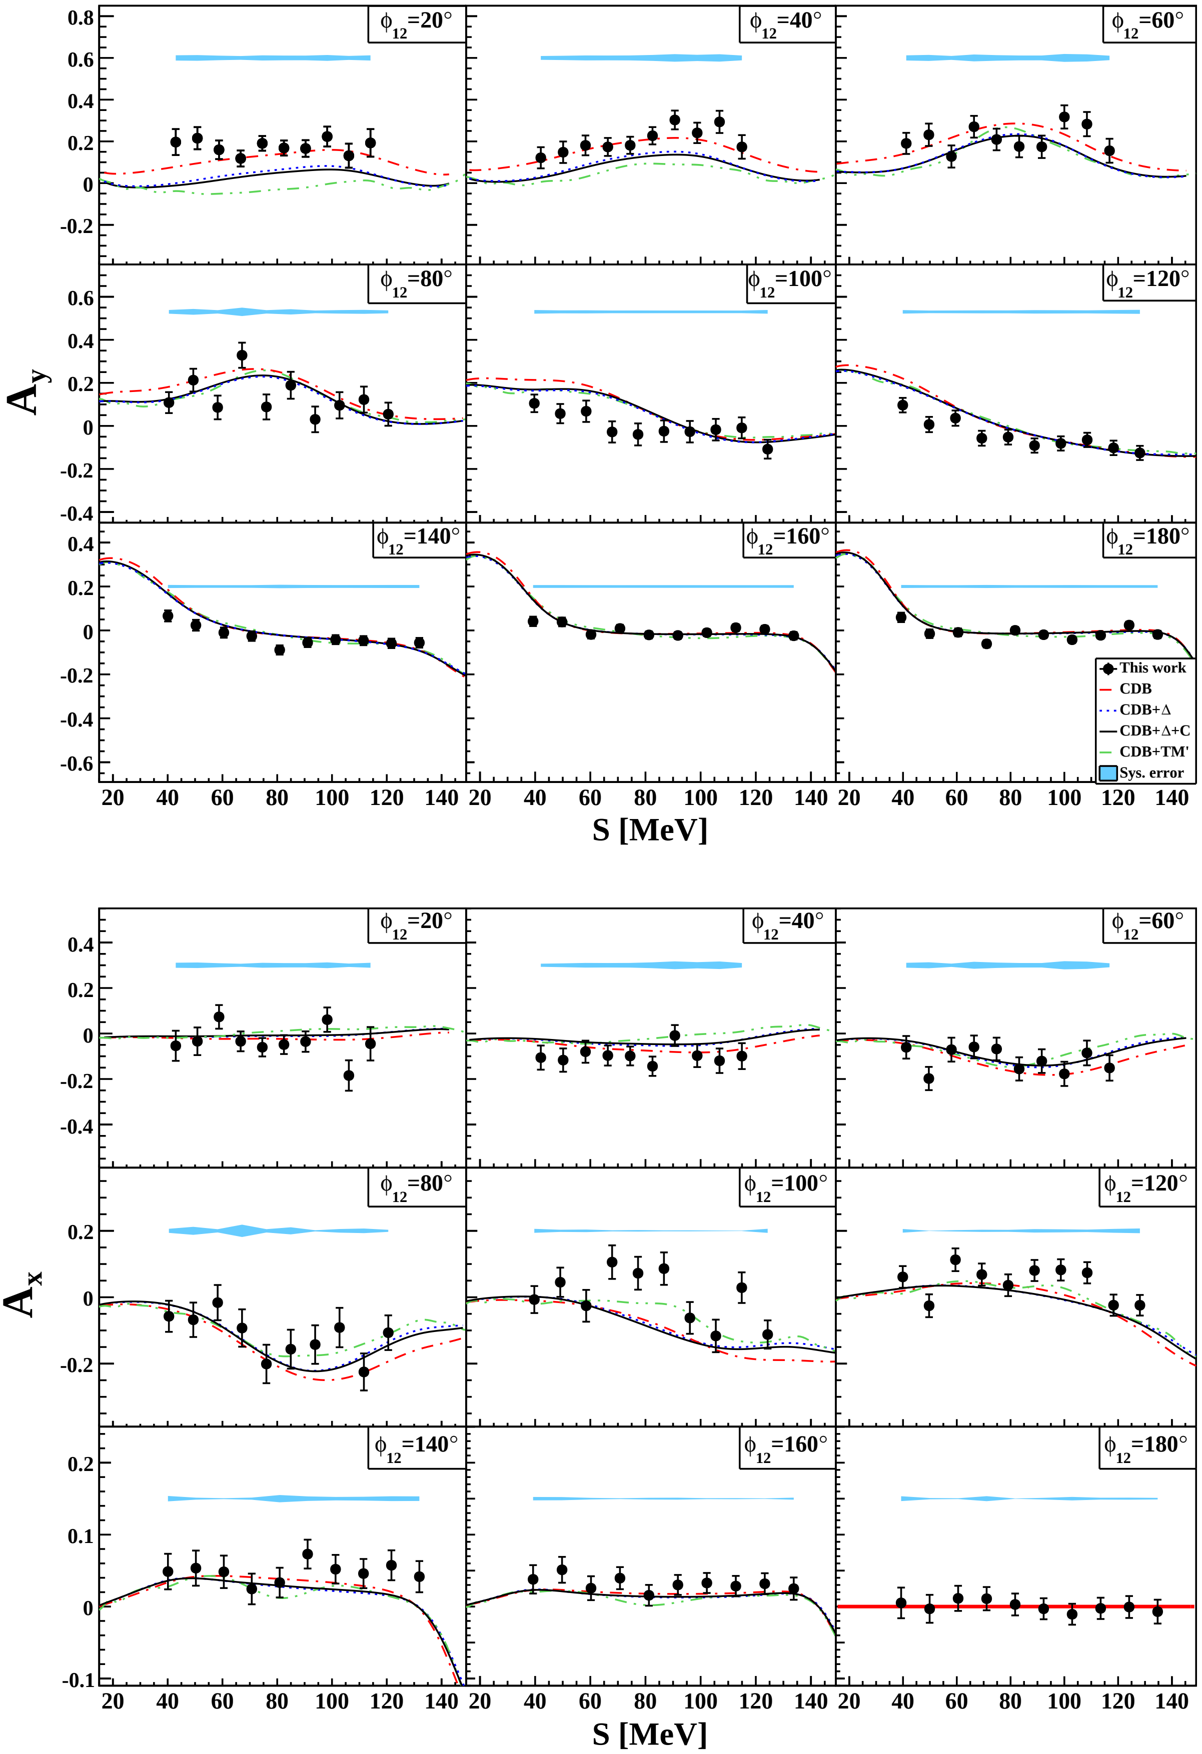


Fig. 16: Same as Fig. 11 except for $(\theta_1, \theta_2) = (24^\circ, 20^\circ)$.

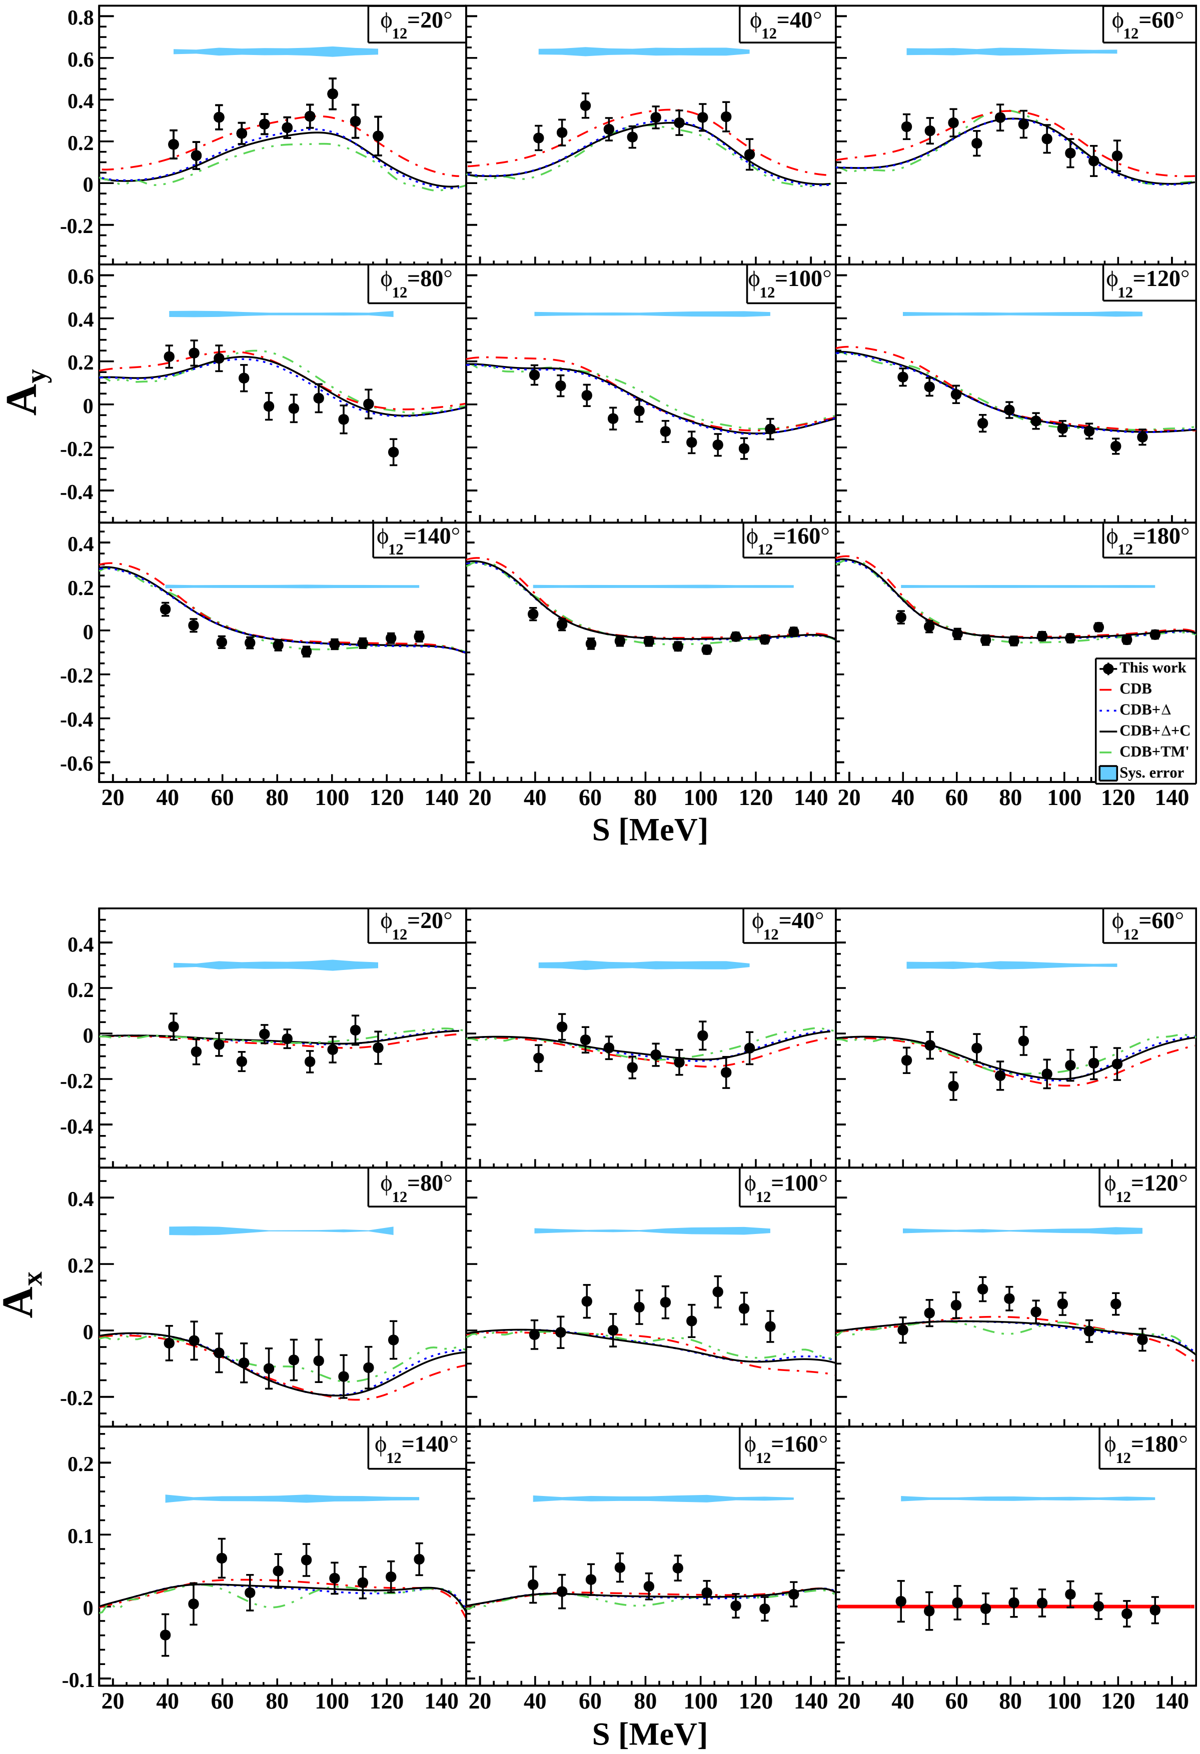


Fig. 17: Same as Fig. 11 except for $(\theta_1, \theta_2) = (24^\circ, 16^\circ)$.

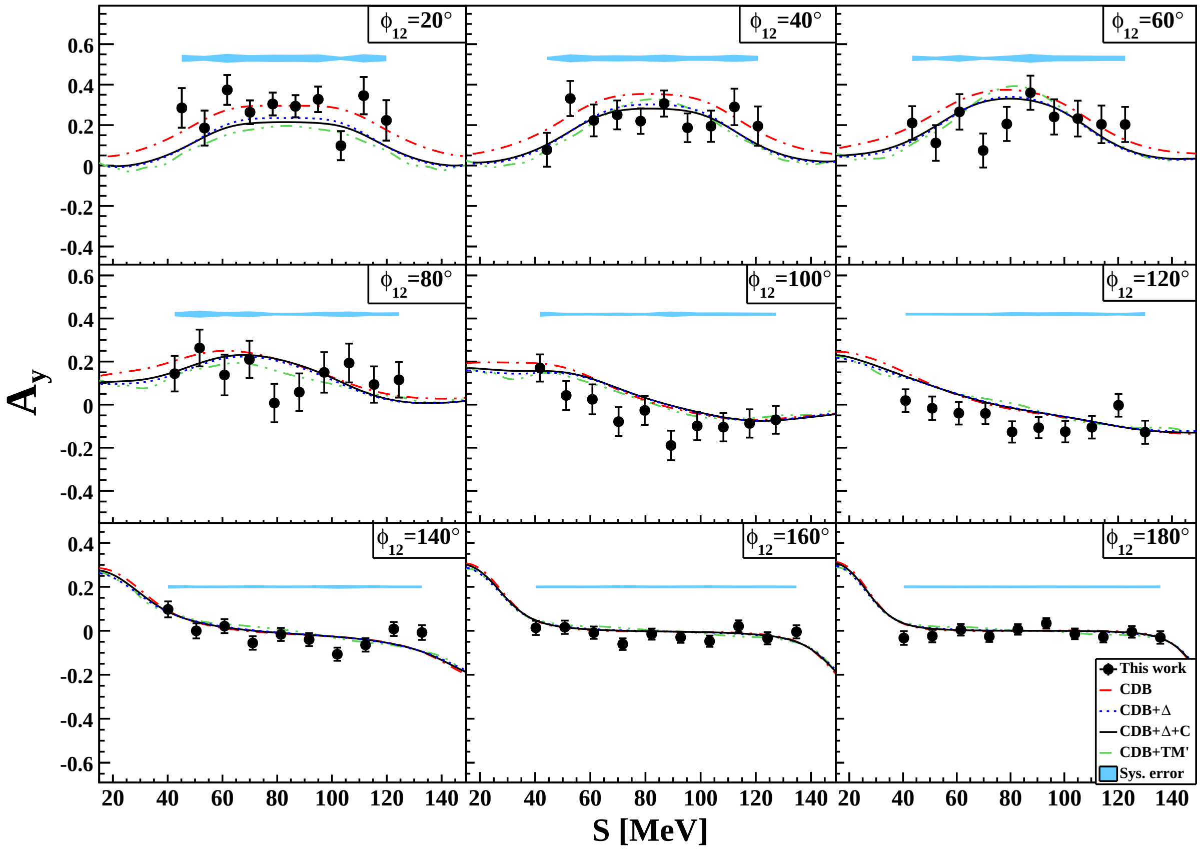


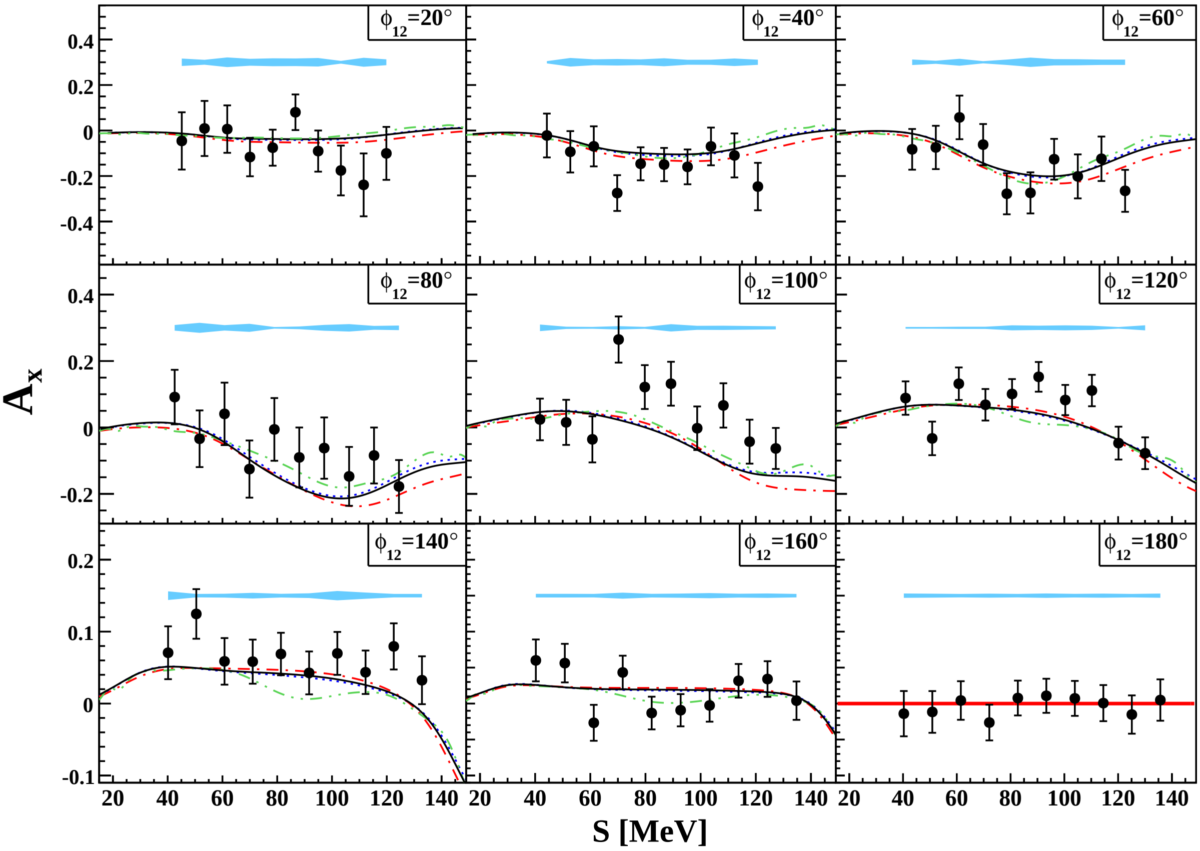


Fig. 18: Same as Fig. 11 except for $(\theta_1, \theta_2) = (20^\circ, 20^\circ)$.

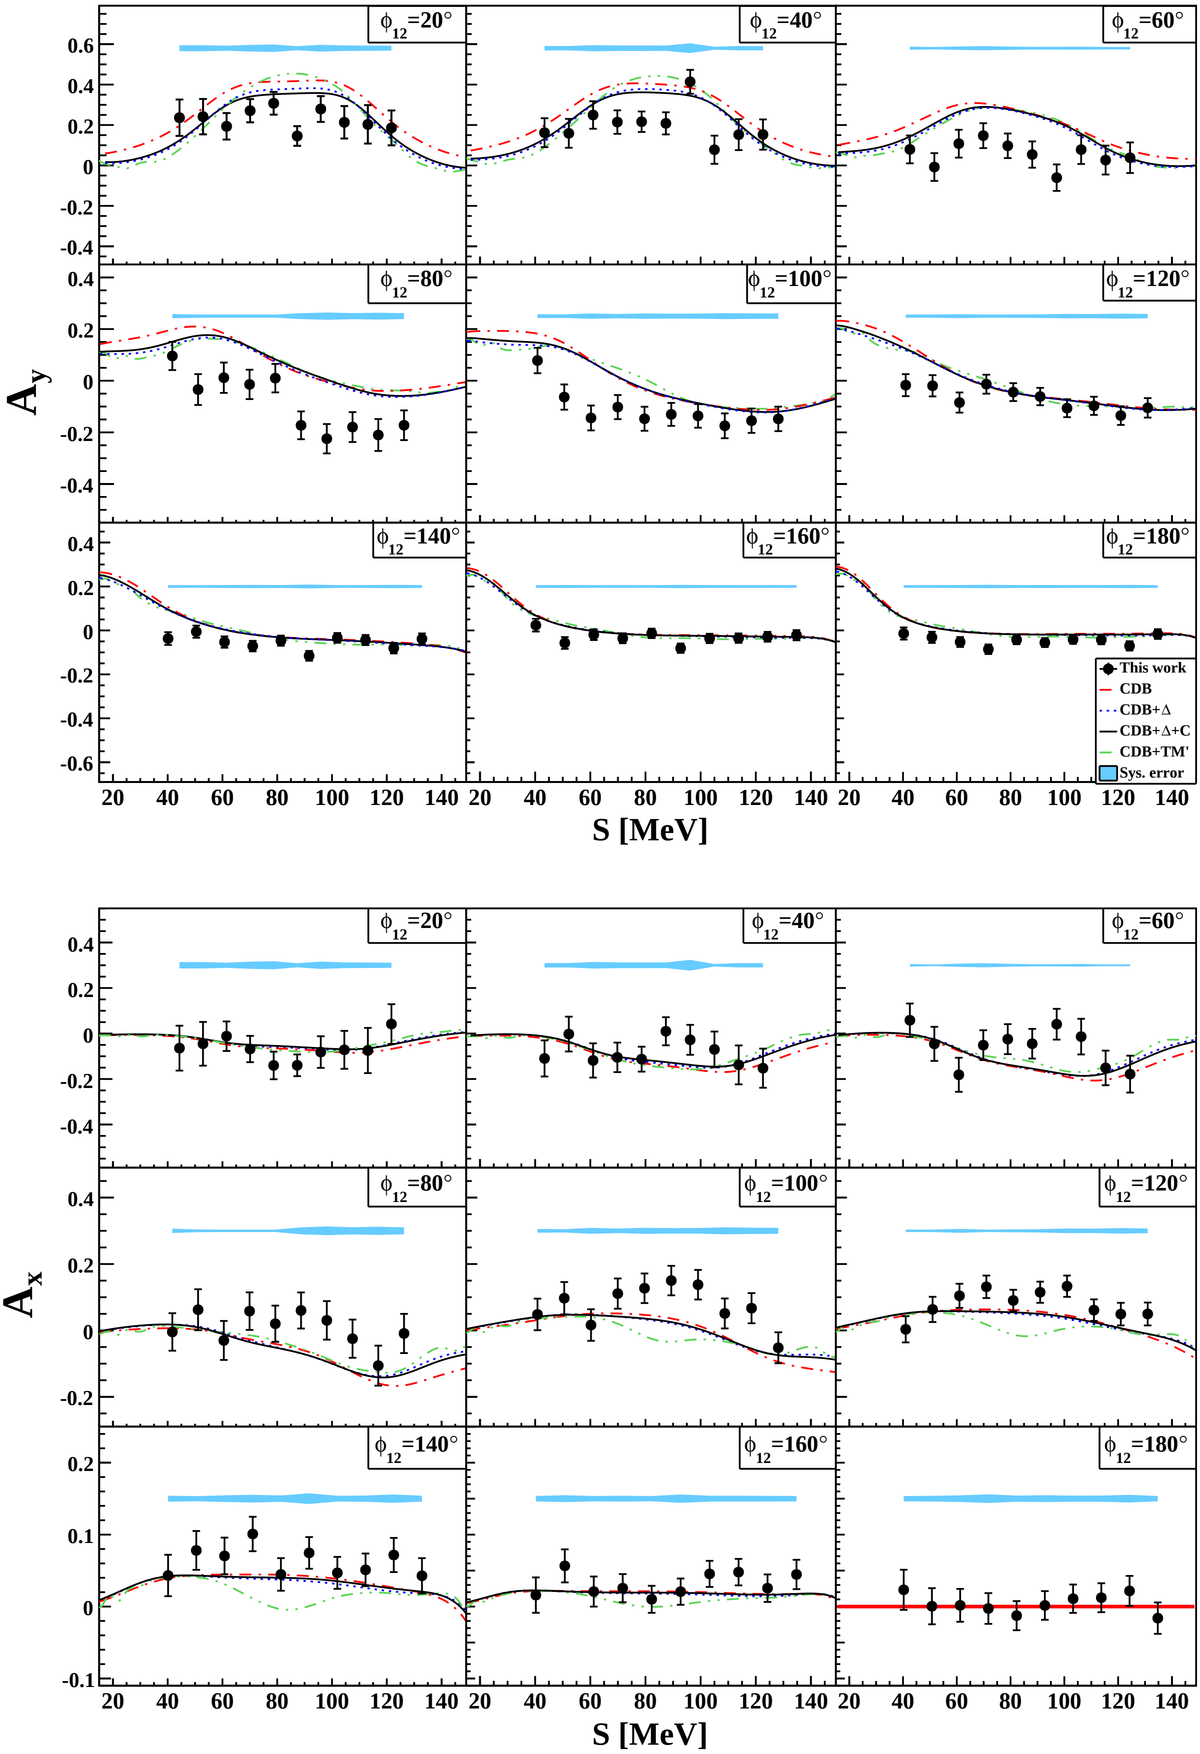


Fig. 19: Same as Fig. 11 except for $(\theta_1, \theta_2) = (20^\circ, 16^\circ)$.

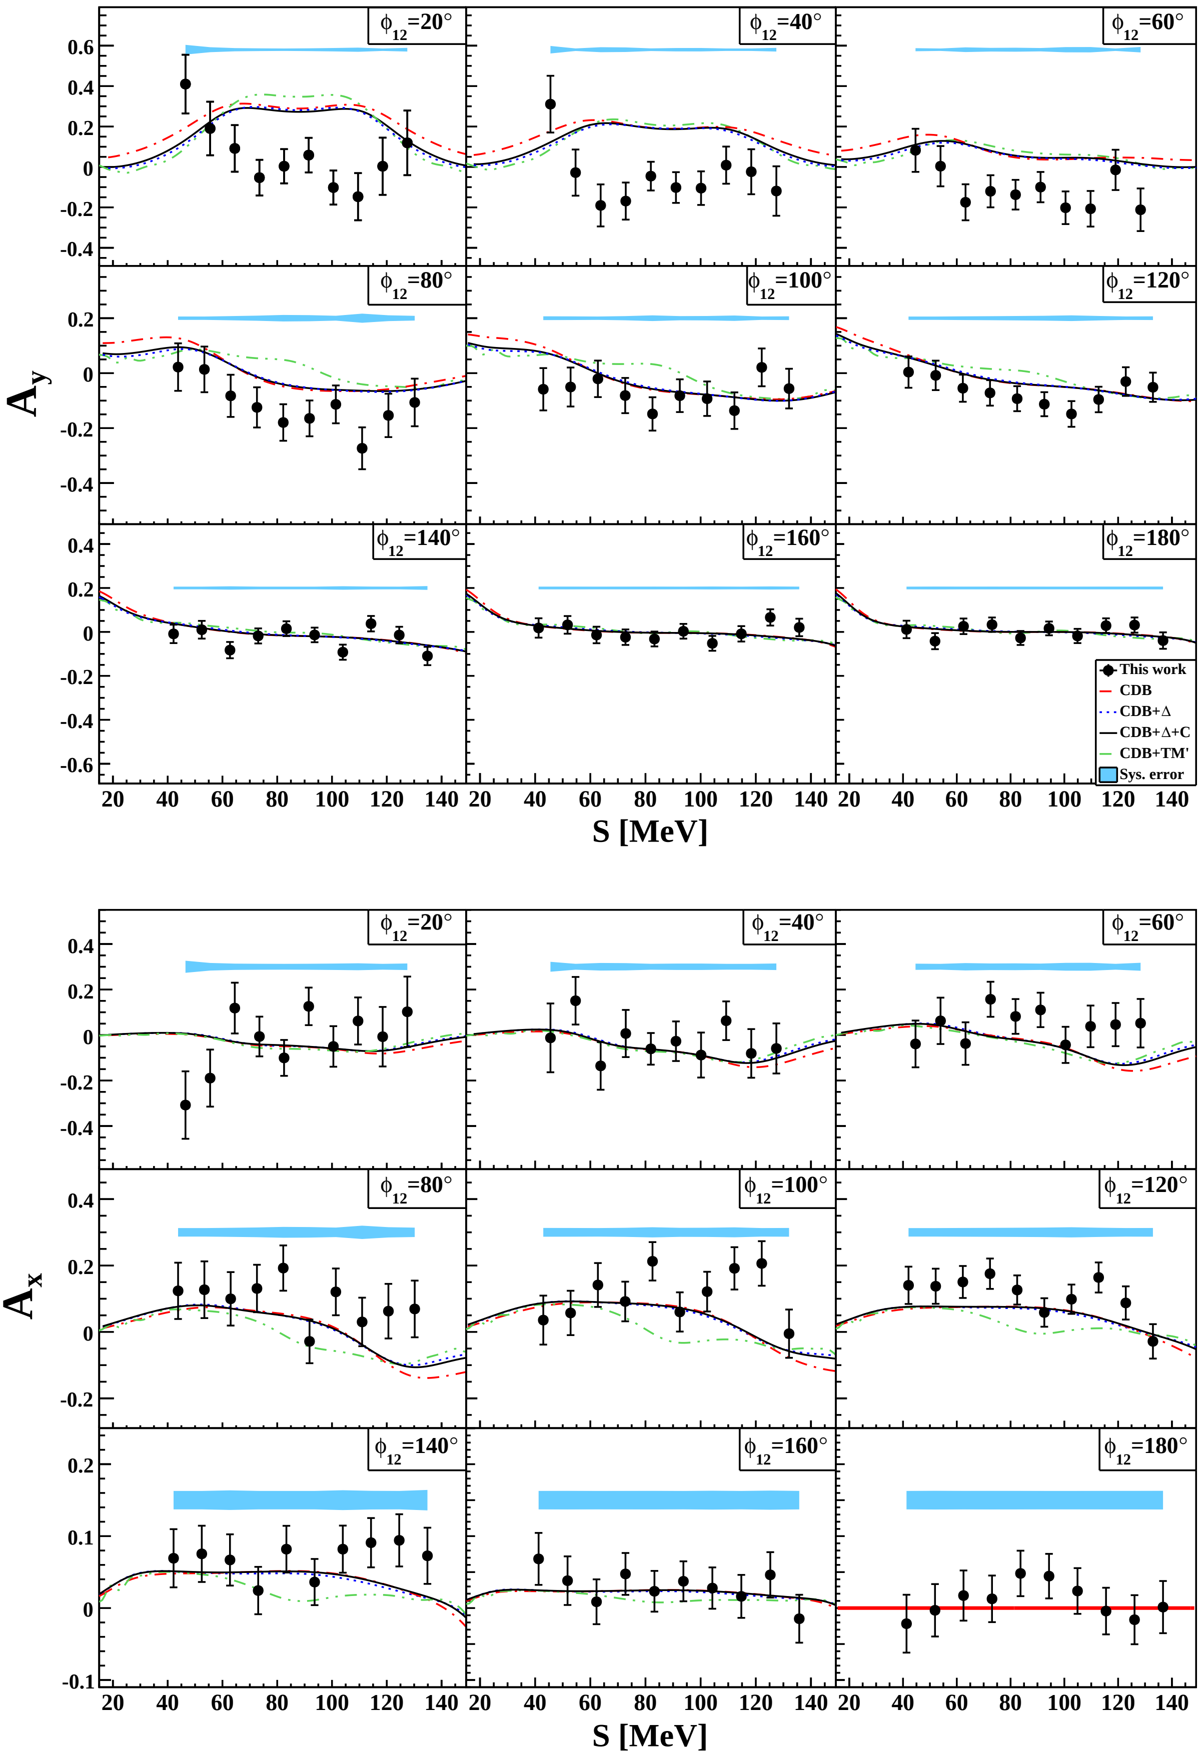


Fig. 20: Same as Fig. 11 except for $(\theta_1, \theta_2) = (16^\circ, 16^\circ)$.

## References

1. A. Deltuva, A.C. Fonseca, P.U. Sauer, Phys. Rev. Lett. **95**, 092301 (2005)
2. A. Deltuva, A. C. Fonseca, P. U. Sauer, Phys. Lett. B **660**, 471 (2008)
3. A. Deltuva, Phys. Rev. C **88**, 011601 (2013)
4. H. Witala, T. Cornelius, W. Glöckle, Few-Body Sys. **3**, 123 (1988)
5. H. Witała, J. Golak, R. Skibiński, W. Glöckle, H. Kamada, A. Nogga, Nucl. Phys. A **827**, 222 (2009),
